# Supplementary material for: Transfer Learning for Improving Model Predictions in Highly Configurable Software
Source: arXiv:1704.00234 source file (2017-04-20)
Supplement: Supplementary file 1 [file appendix.tex]

\section{Appendix}
\label{sec:appendix}
